# Supplementary material for: Recency predicts bursts in the evolution of author citations
Source: arXiv:1911.11926 ancillary file (2019-11-27)
Supplement: Supplementary file 1 [file Supplementary_Information.pdf]

# Supplementary Information

**Recency predicts bursts in author citation dynamics**

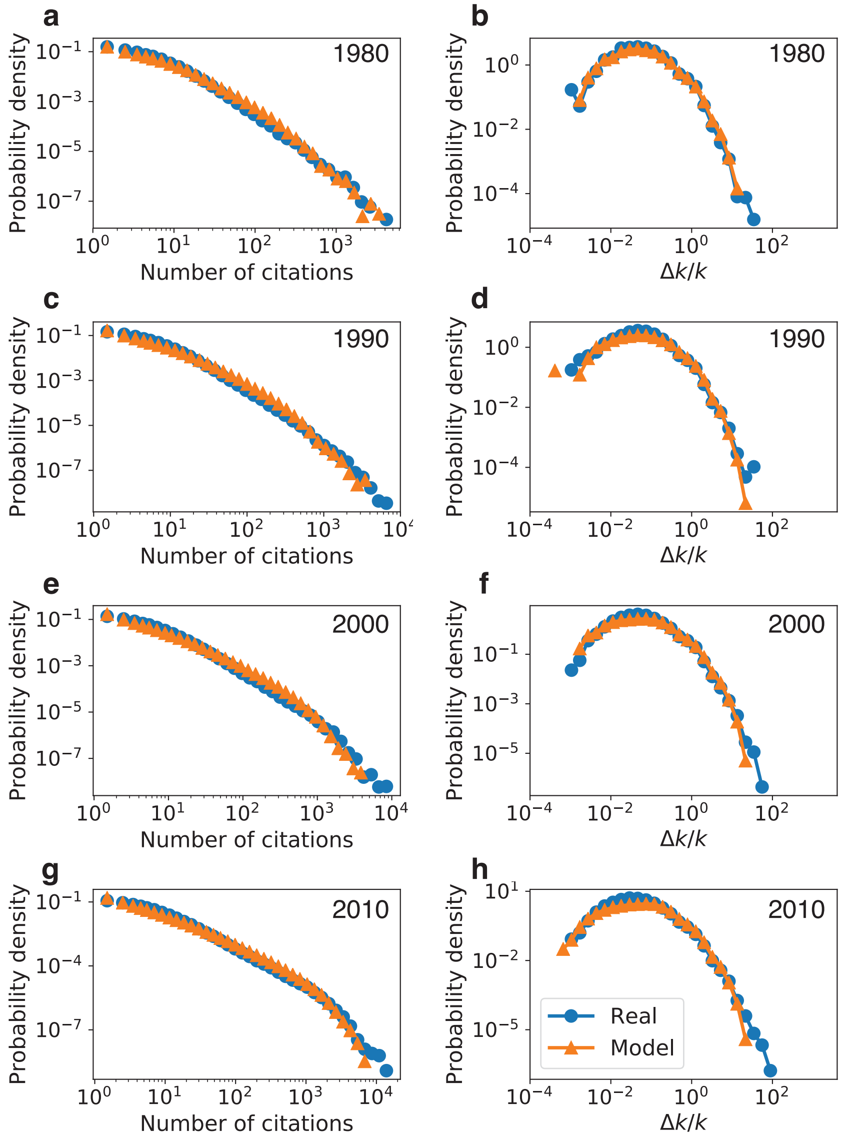


Figure S1: Comparison between empirical and recency model distributions throughout the 1970–2010 period.

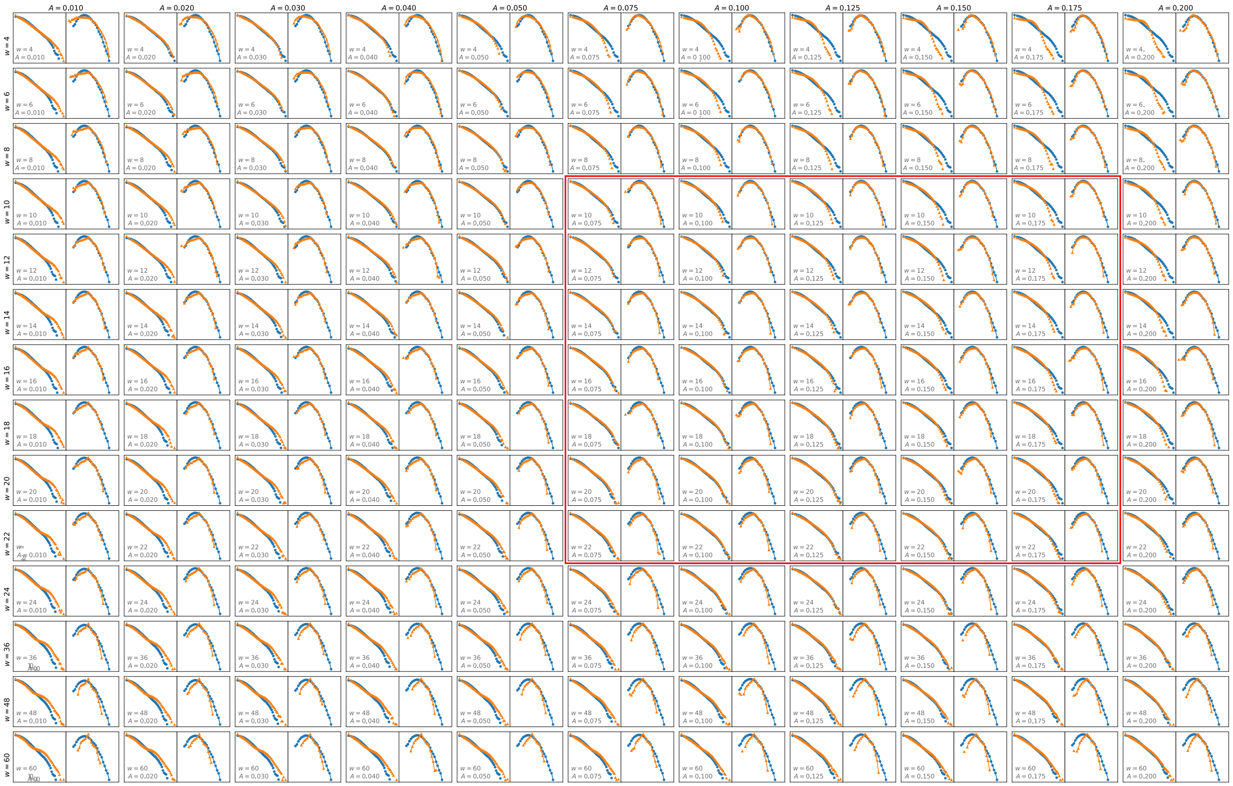


Figure S2: Distribution curves obtained by varying the recency model parameters ($w$ and $A$). Each panel consists of two plots: the citation distribution on the left and the burstiness distribution on the right. Model and empirical curves are shown in orange and blue, respectively. The highlighted region corresponds to the parameter ranges leading to the best fits (Fig. 7).

Table S1: Journals in the APS dataset.

| Journal Name | Publication Period |
|---|---|
| *Physical Review* | 1893–1970 |
| *Reviews of Modern Physics* | 1929–present |
| *Physical Review Letters* | 1958–present |
| *Physical Review A* | 1970–present |
| *Physical Review B* | 1970–present |
| *Physical Review C* | 1970–present |
| *Physical Review D* | 1970–present |
| *Physical Review E* | 1993–present |
| *Physical Review Accelerators and Beams* | 1998–present |
| *Physical Review Physics Education Research* | 2005–present |
| *Physical Review X* | 2011–present |
| *Physical Review Applied* | 2014–present |
| *Physical Review Fluids* | 2016–present |
